# Supplementary material for: Large-Enhancement Nanoscale Dynamic Nuclear Polarization Near a Silicon Nanowire Surface
Source: arXiv:2402.16283 source file (2024-02-26)
Supplement: Supplementary file 1 [file supp.pdf]

# Supplementary Materials for Large-Enhancement Nanoscale Dynamic Nuclear Polarization Near a Silicon Nanowire Surface

Sahand Tabatabaei,[1,2] Pritam Priyadarsi,[1,2] Namanish Singh,[1,2]
Pardis Sahafi,[1,2] Daniel Tay,[1,2] Andrew Jordan,[1,2] Raffi Budakian[1,2*]

[1]Department of Physics and Astronomy, University of Waterloo, Waterloo, ON, Canada, N2L3G1
[2]Institute for Quantum Computing, University of Waterloo, Waterloo, ON, Canada, N2L3G1

[*]To whom correspondence should be addressed; E-mail: rbudakian@uwaterloo.ca.

## 1 Sample Preparation and Attachment

### 1.1 Silicon Nanowire Etching

Before attaching the OX063 samples to the silicon nanowire (SiNW), the Au ball at the nanowire's tip was etched to mitigate potential charge interactions with the CFFGS. An iodine-based etchant, comprising 207 mg KI and 54 mg $I_2$ in 1.43 mL of DI $H_2O$ and 0.36 mL Ethanol, was prepared. Ethanol was added to reduce the surface tension of the solution, a requirement in the subsequent Au etching and sample attachment steps.

A G-1 Narishige glass capillary is pulled into a pipette using the Narishige PC-10 pipette puller. The pipette tip is ground on a Narishige EG-402 micro-grinder until an orifice of approximately 20 μm in diameter is obtained. This pipette is affixed to one arm of the MMO-203 micro-manipulator which is, in turn, connected to the Narishige IM-11-2 pneumatic microinjector. A few drops of the etchant solution were drawn into the pipette. The SiNW and the

capillary tip were aligned under an optical microscope. The etchant was pushed out through the orifice until a curvature was seen. The capillary, guided by the micromanipulator, was moved towards the SiNW and brought in contact with its tip. The reduction in surface tension enabled by the Ethanol allowed for the SiNW tip to penetrate the etchant droplet. This configuration is maintained for up to 2 minutes for complete Au etching. Subsequently, the SiNW tip is cleaned with a 1:1 DI $H_2O$ and Ethanol solution using the micromanipulator and a new glass capillary.

## 1.2 Sample Solution Preparation

To prepare the various OX063 samples, stock solutions with different amounts of constituents were prepared. Table S1 summarizes the constituents for each of the samples.

Table S1: **Constituent table,** including all the components used to prepare the measured samples.

| Constituents | A | B | C | D |
|---|---|---|---|---|
| Sucrose (mg); $C_{12}H_{22}O_{11}$ | - | - | - | 80.7 |
| Glucose (mg); $C_6H_{12}O_6$ | 6.0 | 6.1 | 6.1 | - |
| d-12 Glucose (mg); $C_6D_{12}O_6$ | 54.0 | 54.4 | 54.4 | - |
| $H_2O$ (µL) | 15 | 15 | 15 | 100 |
| $D_2O$ (µL) | 135 | 135 | 135 | - |
| Ethanol (µL) | - | - | - | 50 |
| d-Ethanol (µL) | 150 | 150 | 150 | - |
| OX063 (mg) | 0.92 | 2.58 | 2.58 | 2.10 |
| Concentration (mM) | 17.8 | 49.4 | 49.4 | 29 |

The mixing process began with adding the sugar and the OX063 radicals in the amount given in Table S1 into a 4 mL amber glass vial. Micro-pipettes were then used to pipette the appropriate amount of water into the vial with the sugar and radical mixture. This vial was then pushed onto a vortex shaker to dissolve the sugar and the radicals. Once the dissolution was complete, the appropriate amount of ethanol was pipetted into the mixture, followed by another round on the vortex shaker.

The constituents of the deuterated samples were chosen to ensure a 9:1 ratio of proton to deuterium in the sample (assuming complete evaporation of Ethanol). These ratios were finalized in an attempt to match the concentration ratio of proton to deuterium in DNP juice (*1*).

### 1.3 Sample Attachment

Once the Au etching and cleaning process is completed, the sample is attached to the SiNW tip as follows. The sample solution is drawn into a pointed-tip glass capillary and aligned in front of a SiNW under an optical microscope. Prior to attachment, dry $N_2$ gas is blown over the $20\,\mu m$ diameter orifice of the capillary. The nitrogen flow creates a higher concentration of sugar on the surface of the droplet exiting the capillary, which facilitates the formation of the nano-droplet on the tip of the SiNW. Without the $N_2$ flow, the sample failed to remain attached to the SiNW as the capillary was pulled back.

## 2 CFFGS Fabrication and Field Profile

### 2.1 CFFGS Fabrication

The current-focusing field gradient source (CFFGS) is a lithographically fabricated nanoscale metallic constriction that generates the magnetic field gradients used for spin detection and the magnetic fields used for spin control. Fig. S1A shows an optical image of the CFFGS. The image was constructed by combining multiple optical images and refining them with image editing software. The device is a microstrip transmission line engineered to operate in the X-band. Finite element method simulations using HFSS indicated an insertion loss of 0.7 dB at 9.26 GHz for the device.

The device is fabricated by UHV sputtering a $100\,nm$ thick Al film on a sapphire substrate. The head section of the device, shown in Fig. S1B, is patterned via e-beam lithography and metal reactive ion etching. The remaining section of the leads is thickened to $400\,nm$ by de-

positing an additional Al layer to lower the device's electrical resistance. An SEM image of the thickened layer is shown in Fig. S1C. Lastly, the ground plane of the microstrip is made by depositing a $100\,\mathrm{nm}$ thick Al layer on the back side of the sapphire wafer.

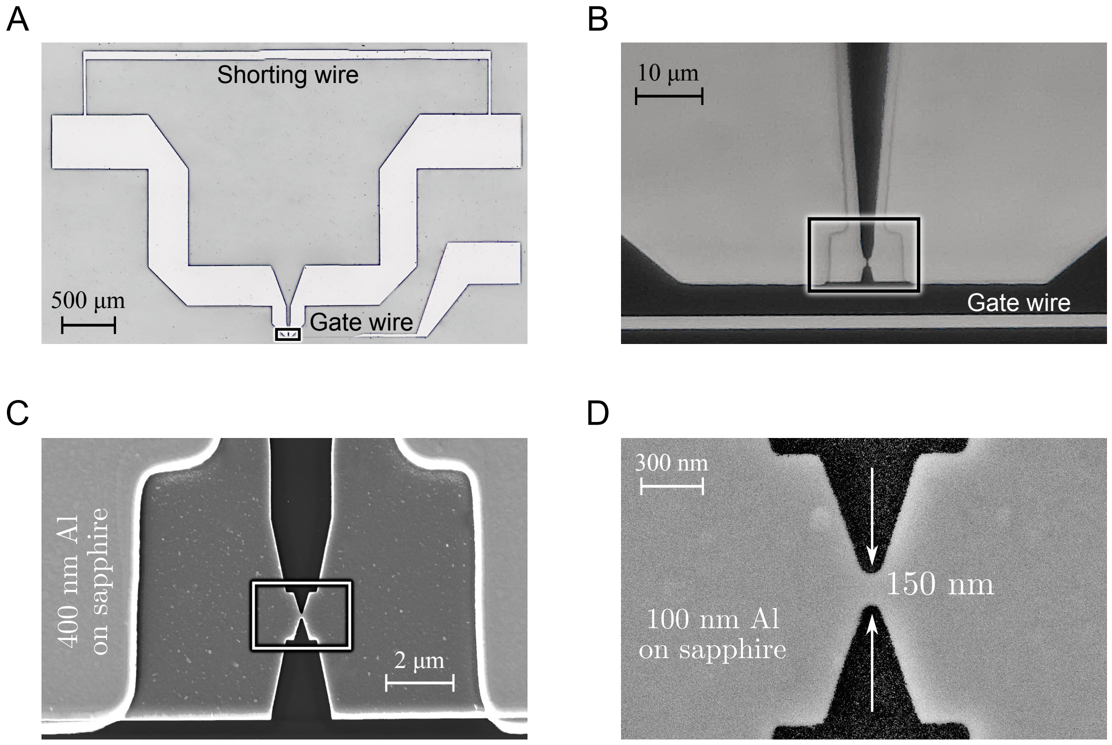


Figure S1: **CFFGS Images.** (**A**) Optical image of the CFFGS. (**B**) Optical image of the head section of the CFFGS. The metal lead on the lower part of the figure is connected to the gate shown in (**A**) used to apply an electrostatic potential to the SiNW. (**C**) SEM of the constriction section of the CFFGS. (**D**) SEM of the constriction.

The shorting wire, seen on the top section of Fig. S1A, is fabricated to prevent electrostatic discharge through constriction during the fabrication processes. The connection is broken by scribing the wire after wire bonding the leads to the PCB carrier. The gate, seen in the lower part of Fig. S1B, is used to mitigate interactions between the CFFGS and charges on the surface of the sample by applying a voltage bias.

## 2.2 Field Profiles

The magnetic field configuration produced by the CFFGS is calculated using the COMSOL finite element simulation software. The simulated Rabi field $B_1(\mathbf{r}) = \sqrt{B_x^2(\mathbf{r}) + B_y^2(\mathbf{r})}/2$ and the detection gradient $G(\mathbf{r}) = \partial B_y(\mathbf{r})/\partial z$ are shown in Fig. S2.

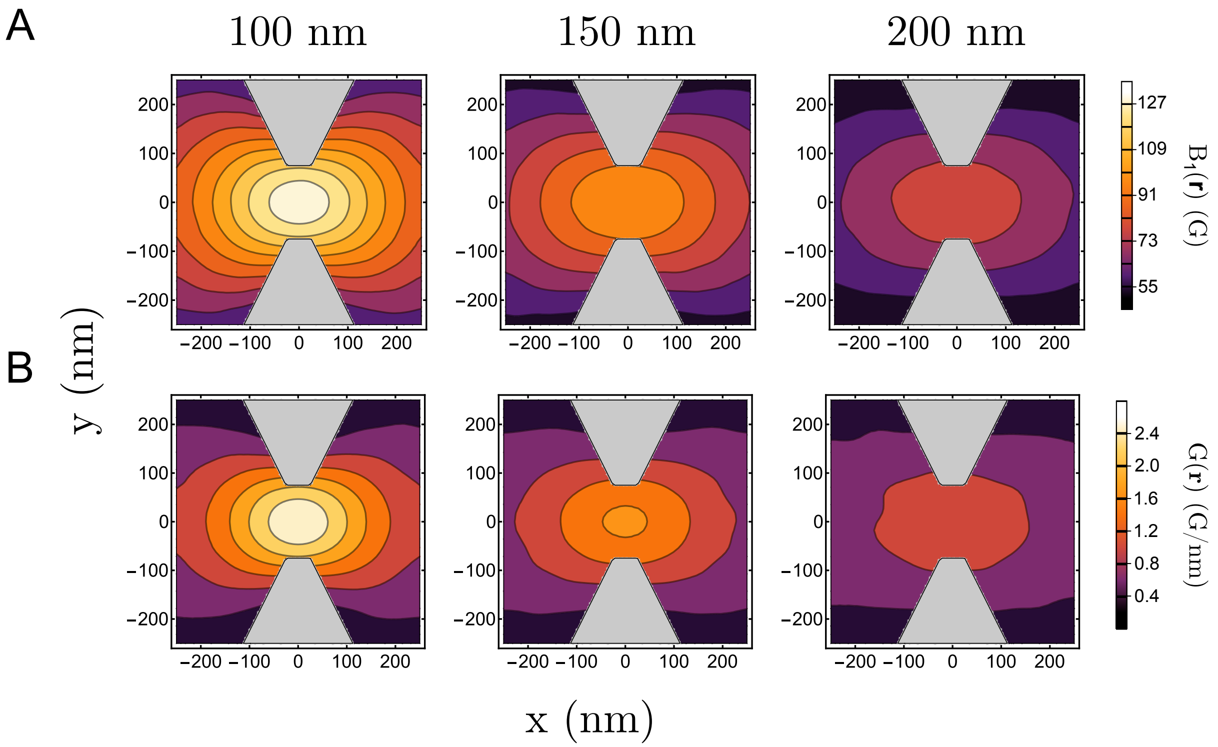


Figure S2: **CFFGS Field Distribution.** (**A**) Simulated Rabi field contours and (**B**) Simulated detection gradient contours at different heights above the center of the CFFGS. The $B_1$ profiles were generated for a peak current of 29 mA while the $G(\mathbf{r})$ profiles were generated for a peak current of 47 mA passing through the CFFGS.

# 3 MAGGIC protocol

Here, we briefly discuss the MAGGIC spin detection protocol, while referring to (*2, 3*) for a detailed description. The modulated alternating gradients generated with currents (MAGGIC) protocol, depicted in Fig. S3, converts the $z$-axis spin magnetization to a resonant force on the

SiNW oscillator. After implementing the spin control sequence of interest e.g., the imaging sequence shown in Fig. 5A in the main text, a measurement block with a duration of $\tau_0$ is applied. The measurement involves the repeated application of the MAGGIC waveform primitive (Fig. S3A), in which we modulate the $G(\mathbf{r}) = \partial B_z(\mathbf{r})/\partial y$ gradient at the SiNW resonance frequency $\omega_c$ by driving a current $I_c(t)$ through the CFFGS. The gradient modulation is phase shifted by $\pi$ between successive MAGGIC waveform primitives to avoid spurious electrical forces at $\omega_c$. The polarization of the spins being measured is inverted between two MAGGIC primitives using an adiabatic full passage (AFP), which combined with the phase shift of the gradient modulation, results in a resonant force

$$\mathcal{F}(t) = \frac{\mu D}{\sqrt{2}} \int d^3r \; n(\mathbf{r})G(\mathbf{r})h(\mathbf{r},t) + \mathcal{N}(t) \tag{S1}$$

at $\omega_c$. Here, $D = \tau_1/(\tau_1 + \tau_2)$ is the duty cycle of the gradient modulation (Fig. S3A), $\mu$ is the spin magnetic moment, $n(\mathbf{r})$ is the spin density at position $\mathbf{r}$, and $\mathcal{N}(t)$ is the oscillator's thermal force noise, which is a stationary white random process. $h(\mathbf{r},t) \in \{-1, 1\}$ is a random telegraph process that models the random evolution of the $z$ projection of the spin during the measurement (*3*). The number of sign flips of $h$ over a given time interval is Poisson distributed, which results in the autocorrelation $\langle h(\mathbf{r},t_1)h(\mathbf{r},t_2)\rangle = e^{-|t_2-t_1|/\tau_m}$. The spin correlation time $\tau_m$ encompasses the combined effect of the AFP infidelity and $T_1$ relaxation during the MAGGIC protocol.

For the enhancement measurements presented in Fig. 4 of the main text, $D = 72.3\%$ ($\tau_1 = 42.28$ $\mu$s, $\tau_2 = 16.17$ $\mu$s), and the measure block duration was $\tau_0 = 200$ ms. For the imaging experiments presented in Fig. 5 of the main text, the duty cycle was increased to $D = 90.2\%$ ($\tau_1 = 154.4$ $\mu$s, $\tau_2 = 16.78$ $\mu$s) to improve the SNR. The measure block duration was also increased to $\tau_0 = 400$ ms to accommodate the larger $\tau_m$ achieved via electron decoupling (Fig. 5 of the main text). The AFP used in the MAGGIC waveform was the numerically-optimized 2.3

Rabi-cycle AFP presented in Ref. (*4*). The AFP was $15.44\,\mu$s long and inverts proton spins with Rabi frequencies $\omega_{1I}/(2\pi) \geq 150\,$kHz.

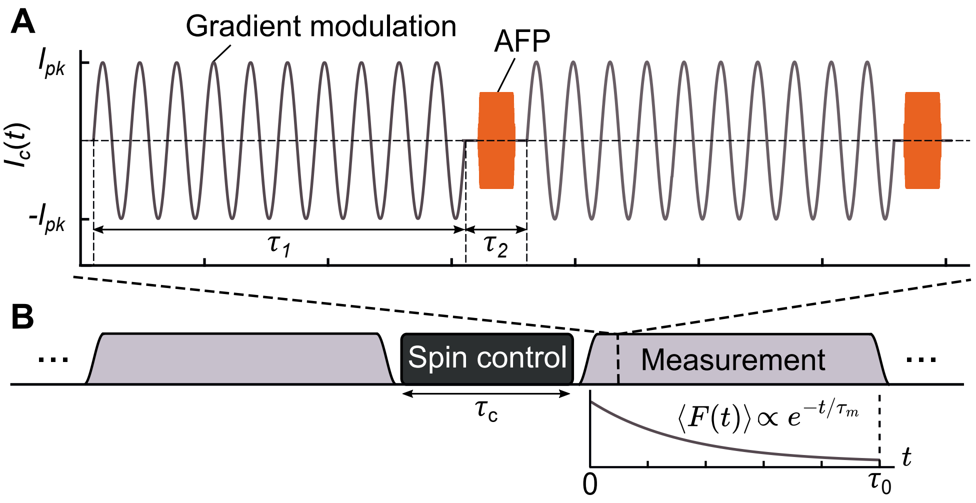


Figure S3: **General Schematic of the MAGGIC Protocol.** (**A**) The MAGGIC waveform primitive. (**B**) A typical nanoscale magnetic resonance experiment, including the spin control and measurement blocks. The spin control block contains the spin control pulses of interest, e.g. imaging pulses, DNP, etc. The MAGGIC waveform generates a resonant force on the spins, which decays exponentially (bottom figure).

## 3.1 Average Polarization Measurements

For measurements using the average polarization, we measure the sample average $F(t) = \sum_{k=1}^{M} \mathcal{F}_i(t)/M$ over $M$ realizations of the force from Eq. S1, where the index $i$ denotes the $i^{\text{th}}$ realization. Each spin builds up an average polarization $m_0(\mathbf{r}) = \langle h(\mathbf{r}, 0)\rangle$ at the start of a measurement block. The associated probability distribution is $\mathbb{P}[h(\mathbf{r}, 0) = \pm 1] = (1 \pm m_0(\mathbf{r}))\,/2$. This, along with the Poisson distribution governing the number of spin flips, determines $\langle h(\mathbf{r}, t)\rangle = m_0(\mathbf{r})e^{-t/\tau_m}$, which results in an expectation value of the force signal equal to

$$\langle F(t)\rangle = \frac{\mu D}{\sqrt{2}} e^{-t/\tau_m} \int d^3r\; n(\mathbf{r})G(\mathbf{r})m_0(\mathbf{r}). \tag{S2}$$

This exponentially decaying force resonant with the SiNW translates to a mean displacement

$$\langle Y(t)\rangle = \frac{\mu D Q_c}{\sqrt{2}k}\,\frac{e^{-t/\tau_m} - e^{-t/\tau_Q}}{1-\tau_Q/\tau_m}\int d^3r\; n(\mathbf{r})G(\mathbf{r})m_0(\mathbf{r}), \tag{S3}$$

which is detected with optical interferometry. Here, $k$ is the spring constant, $Q_c \sim 900$ is the damped quality factor, and $\tau_Q = 2Q_c/\omega_c \sim 1$ ms is the characteristic response time of the oscillator. Since $\tau_m \gg \tau_Q$, we have $\langle Y(t)\rangle \simeq (Q_c/k)\langle F(t)\rangle$ for $t \gg \tau_Q$, i.e. the measured displacement is proportional to the force, apart from the fast initial rise in the signal due to the oscillator's finite bandwidth. Eq. S3 is the model used for the fits in Fig 4B of the main text.

We process the acquired force record $F(t)$ using a matched filtering scheme for optimal SNR (*5*). Assuming the noise in the measured $F(t)$ is approximately white, we seek a kernel $w(t)$, for which the inner product $\bar{F} = \langle w|F\rangle = \int_0^{\tau_0} dt\; w(t)F(t)$ maximizes the $\mathrm{SNR} = \langle\bar{F}\rangle/\sqrt{\mathrm{Var}(\bar{F})} \propto \langle w|F\rangle/\|w\|$. Here, $\mathrm{Var}(\bar{F})$ denotes the variance of $\bar{F}$. By the Cauchy-Schwartz inequality, the optimal kernel is $w(t) \propto F(t)$. Therefore, we fit a function of the form Eq. S3 to the measured hyperpolarized $F(t)$ of each sample, and use it for $w(t)$. We then normalize $w(t)$ such that $\int_0^{\tau_0} dt\; w(t) = 1$ to ensure that $\bar{F}$ can be interpreted as a weighted average of $F(t)$. Since $\tau_Q \ll \tau_0, \tau_m$, we can neglect the fast initial rise in Eq. S3, and approximately take $w(t) \propto e^{-t/\tau_m}$. This, along with Eq. S2 gives the average matched-filter output

$$\langle\bar{F}\rangle = \frac{\mu D}{2\sqrt{2}}(1 + e^{-\tau_0/\tau_m})\int d^3r\; n(\mathbf{r})G(\mathbf{r})m_0(\mathbf{r}). \tag{S4}$$

For a calculation of the fluctuations around this mean value, and the corresponding detection SNR, see Section 4.

## 3.2 Statistical Polarization Measurements

For measurements using statistical polarization, we construct a correlation function between the time-averaged $\mathcal{F}(t)$ force signal between adjacent measurement blocks:

$$C = \frac{1}{M-1} \sum_{i=1}^{M-1} \bar{F}_i \bar{F}_{i+1}, \tag{S5}$$

where $\bar{F}_i$ is the time-average of $\mathcal{F}$ over the $i^{\text{th}}$ measurement block. For statistical polarization measurements, $\bar{F}_i$ is calculated with uniform weighting, i.e. $w(t) = 1/\tau_0$. The average correlation $\langle C \rangle$ is (*2, 3*)

$$\langle C \rangle = \frac{\mu^2 D^2}{2} e^{-\tau_c/\tau_m} \left( \frac{\tau_m}{\tau_0} \right)^2 \left( 1 - e^{-\tau_0/\tau_m} \right)^2 \int d^3 r \; n(\mathbf{r}) G^2(\mathbf{r}) \zeta(\mathbf{r}), \tag{S6}$$

where $\tau_c$ is the duration of the spin control block, and $\zeta(\mathbf{r}) = \mathrm{Tr}[\sigma_z \varrho_f(\mathbf{r})]$ is the proportional to the expectation value of the $z$ component of the spin, and $\varrho_f(\mathbf{r})$ is the reduced density matrix of a spin at position $\mathbf{r}$, which is the result of evolution under the spin control block starting from the $|\uparrow\rangle$ state. For a calculation of the fluctuations in the measured correlation $C$, and the corresponding detection SNR, see Section 4.

Importantly, comparing Eq. S6 to Eq. S4 shows that the signal contribution from each spin is weighted by the square of the detection gradient $G^2(\mathbf{r})$ for statistical polarization measurements, whereas average polarization measurements have a $G(\mathbf{r})$ weighting. Therefore, the effective detection volume for statistical measurements is smaller, and more confined to near the CFFGS surface. Fig. S4 illustrates this by showing the simulated spatial distribution of the hyperpolarized and statistical signals using the geometry of sample A, and the simulated CFFGS field gradients given in Section 2.2.

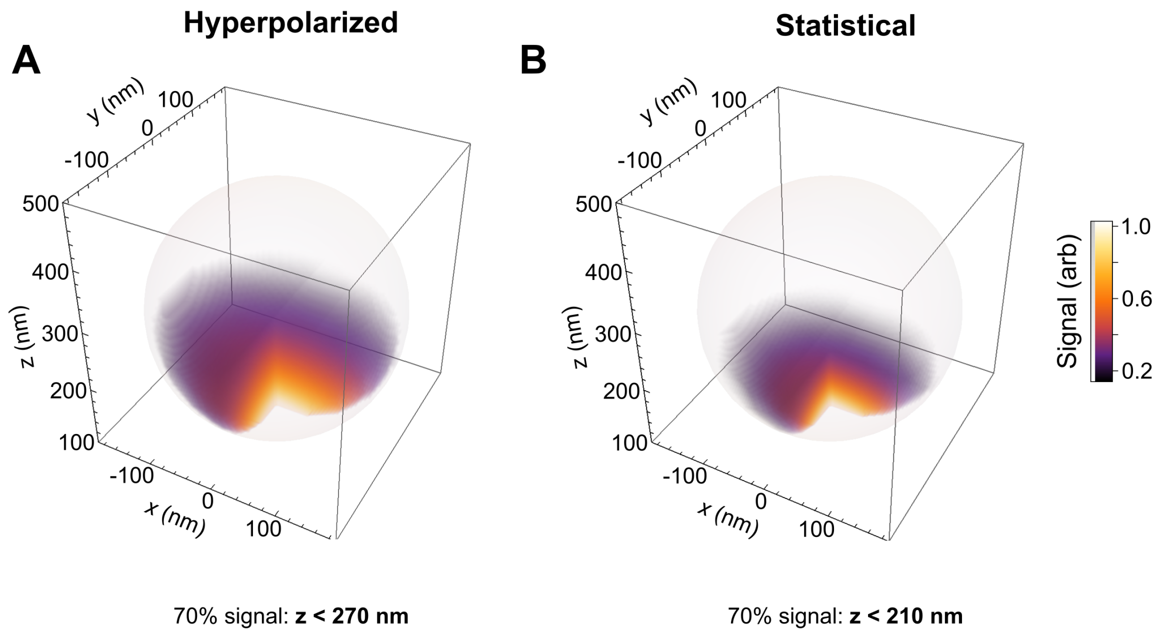


Figure S4: **Effective Detection Volume for Statistical and Hyperpolarized Measurements.** Simulated spatial distribution of the proton signal for the Sample A geometry using (**A**) hyperpolarized and (**B**) statistical polarization measurements. The signal is more confined to the tip for the statistical measurement due to the $G^2(\mathbf{r})$ weighting in the correlation signal (Eq. S6). The volume corresponding to 70% of the full signal is $(240\ \mathrm{nm})^3$ and $(195\ \mathrm{nm})^3$ for the hyperpolarized and statistical signals, respectively. The total volume of the sample is $(301\ \mathrm{nm})^3$.

# 4 Theoretical SNR Comparison of Statistical and Average Polarization Measurements

In this section, we provide a detailed theoretical comparison of the SNR for measuring the average and statistical polarization using the MAGGIC protocol. The dominant sources of noise in force-detected nanoMRI platforms are 1) thermal force noise from the nanomechanical oscillator, and 2) random fluctuations of the spin polarization, i.e. spin noise. In the following, we calculate the variance of the average spin force $\bar{F}$ and spin correlation $C$ due to these two noise sources.

**Average Polarization Measurements**

Assuming statistically independent acquisitions, $\mathrm{Var}(\bar{F})$ is calculated using Eq. S1

$$\begin{aligned}\mathrm{Var}(\bar{F}) &= \mathrm{Var}\left(\frac{1}{M}\sum_{i=1}^{M}\int_0^{\tau_0} dt\, w(t)\mathcal{F}_i(t)\right)\\ &= \frac{\mu^2 D^2}{2M}\int d^3r\, n(\mathbf{r})G^2(\mathbf{r})\int_0^{\tau_0} dt_1\int_0^{\tau_0} dt_2\, w(t_1)w(t_2)\mathrm{Cov}\left[h(\mathbf{r},t_1),h(\mathbf{r},t_2)\right] + \frac{S_F}{2M}\|w\|^2,\end{aligned} \tag{S7}$$

where $h(\mathbf{r},t)$ is assumed to be uncorrelated for the different spins, and $S_F = 4k_BkT/(\omega_c Q)$ is the single-sided power spectral density of the oscillator force noise $\mathcal{N}(t)$. Here, $Q$ is the native (undamped) quality factor of the oscillator. Since $m_0(\mathbf{r}) \ll 1$, $\mathrm{Cov}[h(\mathbf{r},t_1),h(\mathbf{r},t_2)] \approx \langle h(\mathbf{r},t_1)h(\mathbf{r},t_2)\rangle = e^{-|t_2-t_1|/\tau_m}$, which, along with $w(t)\propto e^{-t/\tau_m}$, results in

$$\mathrm{Var}(\bar{F}) = \frac{\tau_0+\tau_c}{T_e}\left[\frac{\mu^2D^2}{4}\frac{\left(1-e^{-2\tau_0/\tau_m}\right)-2\frac{\tau_0}{\tau_m}e^{-\frac{2\tau_0}{\tau_m}}}{\left(1-e^{-\tau_0/\tau_m}\right)^2}\int d^3r\, n(\mathbf{r})G^2(\mathbf{r}) + \frac{S_F}{4\tau_m}\frac{1+e^{-\tau_0/\tau_m}}{1-e^{-\tau_0/\tau_m}}\right], \tag{S8}$$

with $T_e = M(\tau_0+\tau_c)$ being the total experiment duration.

**Statistical Polarization Measurements**

To calculate the fluctuations in the correlation $C$ from Eq. S5, we follow a method similar to Ref. (*6*). This is done in the absence of a spin control block, i.e. $\zeta(\mathbf{r}) = 1$. We write the time-averaged force signal of the $i^{\mathrm{th}}$ measurement block as $\bar{F}_i = \bar{f}_i + \bar{\mathcal{N}}_i$, where $\bar{f}_i$ and $\bar{\mathcal{N}}_i$ denote the contributions of the spin and oscillator force noise, respectively. We thus have $C = C_{ff}+C_{fn}+C_{nf}+C_{nn}$, where

$$C_{ff} = \frac{1}{M-1}\sum_{i=1}^{M-1}\bar{f}_i\bar{f}_{i+1}, \qquad C_{fn} = \frac{1}{M-1}\sum_{i=1}^{M-1}\bar{f}_i\bar{\mathcal{N}}_{i+1},$$
$$C_{nf} = \frac{1}{M-1}\sum_{i=1}^{M-1}\bar{\mathcal{N}}_i\bar{f}_{i+1}, \qquad C_{nn} = \frac{1}{M-1}\sum_{i=1}^{M-1}\bar{\mathcal{N}}_i\bar{\mathcal{N}}_{i+1},$$

It is straightforward to check that all four terms are pairwise uncorrelated. Hence, $\mathrm{Var}(C) = \mathrm{Var}(C_{ff}) + \mathrm{Var}(C_{fn}) + \mathrm{Var}(C_{nf}) + \mathrm{Var}(C_{nn})$. The first and last terms capture fluctuations in the sample correlation due to spin noise and oscillator noise, respectively, while the other two terms encompass the covariance between the two. Each term is calculated using standard formulae for the variance of the sample autocovariance and cross-covariance functions in the $M \gg 1$ limit (*7, 8*). For the first term, this gives

$$\mathrm{Var}(C_{ff}) = \frac{1}{M} A\Big(\frac{\tau_0}{\tau_m}, \frac{\tau_c}{\tau_m}\Big)\sigma_f^4, \tag{S9}$$

where

$$\sigma_f^2 \equiv \mathrm{Var}(\bar{f}_i) = \mu^2 D^2 \left(\frac{\tau_m}{\tau_0}\right)\left(1 - (1 - e^{-\tau_0/\tau_m})\frac{\tau_m}{\tau_0}\right) \int d^3r \; n(\mathbf{r}) G^2(\mathbf{r}) \tag{S10}$$

is the variance of the time-averaged spin signal, and $A$ is the dimensionless function

$$A(u,v) \equiv 1 + \frac{(e^u - 1)^2}{4(e^{2(u+v)} - 1)\left(1 + (u-1)e^u\right)^2} \times \\ \left[2\left(e^u - 1\right)^2 + \left(e^u - 1\right)^2\left(1 + e^{-2(u+v)}\right) + 4\left(1 + (u-1)e^u\right)\left(1 - e^{-2(u+v)}\right)\right]. \tag{S11}$$

Similarly,

$$\mathrm{Var}(C_{fn}) = \frac{\mathrm{Var}(\bar{f}_i)\mathrm{Var}(\bar{\mathcal{N}}_i)}{M} = \frac{S_F \sigma_f^2}{2M\tau_0}, \tag{S12}$$

and

$$\mathrm{Var}(C_{nn}) = \frac{\mathrm{Var}(\bar{\mathcal{N}}_i)^2}{M} = \frac{S_F^2}{4\tau_0^2 M}. \tag{S13}$$

Putting Eq. S9,S12,S13 together, and using the fact that $\mathrm{Var}(C_{nf}) = \mathrm{Var}(C_{fn})$ and $M = T_e/(\tau_0 + \tau_c)$, we finally get

$$\mathrm{Var}(C) = \frac{\tau_c + \tau_0}{T_e}\left[A\Big(\frac{\tau_0}{\tau_m}, \frac{\tau_c}{\tau_m}\Big)\sigma_f^4 + \frac{S_F \sigma_f^2}{\tau_0} + \frac{S_F^2}{4\tau_0^2}\right]. \tag{S14}$$

### SNR Comparison

Using the above results, we can compare the detection SNR between hyperpolarized and statistical measurements of proton spins. In the hyperpolarized case, we calculate $\mathrm{SNR}_{\mathrm{hp}} = \langle \bar{F} \rangle / \sqrt{\mathrm{Var}(\bar{F})}$ by combining Eq. S4,S8, assuming uniform proton density, and using the fact that $\tau_c = T_b \gg \tau_0 \gg \tau_m$. This gives

$$\mathrm{SNR}_{\mathrm{hp}} \approx \sqrt{\frac{T_e}{2T_b}} \frac{N\epsilon p_T \mu D \overline{G}}{\sqrt{N\mu^2 D^2 \overline{G^2} + S_F/\tau_m}}, \tag{S15}$$

where $N$ is the number of proton spins, $p_T = \hbar\omega_{0I}/(2k_B T)$ is the proton thermal polarization, $\epsilon$ is the polarization enhancement, and $\overline{G}$ and $\overline{G^2}$ are the average values of $G(\mathbf{r})$ and $G^2(\mathbf{r})$ over the sample volume, respectively.

In the case of statistical polarization measurements, the final expression for $\mathrm{SNR}_{\mathrm{st}} = \langle C \rangle / \sqrt{\mathrm{Var}(C)}$ is rather complicated. To compare with the hyperpolarized case, we instead work with an upper bound for $\mathrm{SNR}_{\mathrm{st}}$, which we construct using the fact that $A(\tau_0/\tau_m,\ \tau_c/\tau_m)\sigma_f^4 + S_F\sigma_f^2/\tau_0 + S_F^2/(4\tau_0^2) \geq A(\tau_0/\tau_m,\ \tau_c/\tau_m)\sigma_f^4$. This, along with $\tau_c \ll \tau_0$, results in the bound

$$\mathrm{SNR}_{\mathrm{st}} \leq \frac{1}{2}\sqrt{\frac{T_e}{\tau_m}} \frac{(1 - e^{-\tau_0/\tau_m})^2}{\sqrt{\frac{\tau_0}{\tau_m} A\left(\frac{\tau_0}{\tau_m}, 0\right) \left[\frac{\tau_0}{\tau_m} - 1 + e^{-\tau_0/\tau_m}\right]}}, \tag{S16}$$

The largest value the right hand side can take across different $\tau_0/\tau_m$ is $\sqrt{2}$. This gives the final upper bound on the statistical SNR:

$$\mathrm{SNR}_{\mathrm{st}} \leq \sqrt{\frac{T_e}{2\tau_m}}. \tag{S17}$$

Combining Eq. S15,S17 gives the sufficient condition $\epsilon > \epsilon_b$ for $\mathrm{SNR}_{\mathrm{hp}} > \mathrm{SNR}_{\mathrm{st}}$, where

$$\epsilon_b = \frac{1}{p_T}\sqrt{\frac{T_b}{\tau_m}\frac{1}{N}\left(\frac{\overline{G^2}}{\overline{G}^2}\right) + \frac{T_b S_F}{2\tau_m^2 N^2 \mu^2 \overline{G}^2}}, \tag{S18}$$

where we also assumed $D \approx 1$. An enhancement larger than $\epsilon_b$ will guarantee a higher SNR when using DNP, irrespective of the details of the measurement protocol.

In Fig. S5B, we provide the calculated $\epsilon_b$ from Eq. S17 for the samples presented in this work, along with the utilized parameters. The average gradient $\overline{G}$ and gradient squared $\overline{G^2}$ were calculated using the simulated CFFGS field distribution (Section 2.2), and $S_F$ was estimated using the measured frequency, quality factor and spring constant for each SiNW. The number of protons was estimated using the calculated proton density and the sample volume. All other parameters are taken from Table 1 of the main text.

**A**

| **Sample** | **A** | **B** | **C** | **D** |
|---|---|---|---|---|
| $\overline{G}$ (G/nm) | 0.66 | 1.19 | 0.59 | 0.62 |
| $\overline{G^2}$ (G$^2$/nm$^2$) | 0.59 | 1.57 | 0.49 | 0.53 |
| $S_F^{1/2}$ (aN/$\sqrt{\text{Hz}}$) | 1.8 | 1.6 | 2.4 | 1.0 |
| $N$ ($\times 10^6$) | 165 | 12 | 227 | 1,878 |
| $\epsilon_b$ | 12.7 | 58.1 | 11.6 | 5.9 |

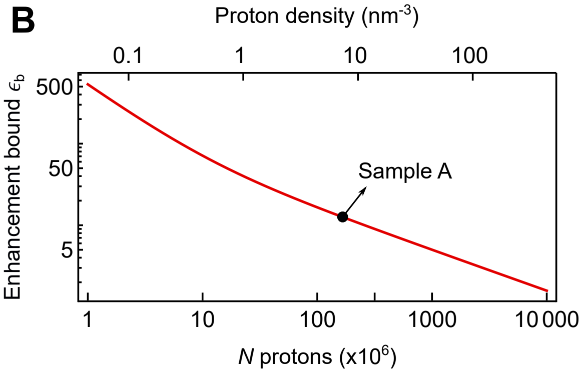


Figure S5: **Calculated Lower Bound on the Polarization Enhancement $\epsilon_b$.** (**A**) Parameters used in the calculation, and the resulting $\epsilon_b$ for the different samples. (**B**) Calculated $\epsilon_b$ as a function number of protons, assuming the same parameters as sample A. The number of protons is varied by changing the spin density while the sample volume (and hence $\overline{G}$, $\overline{G^2}$) is held constant. A DNP enhancement above $\epsilon_b$ guarantees an SNR-advantage over measuring statistical polarization. The black dot in subfigure B corresponds to the calculated proton density for sample A, assuming no remaining water in the sugar droplet.

# 5 Spin Relaxation Measurements

The electron spin and proton spin relaxation times were characterized for all the samples used in the experiment. Here, we present the measured data for sample A, while referring to Table S2 for the other samples. These include the longitudinal and transverse relaxation times for protons $T_{1p}$, $T_{2p}^*$, $T_{2p}$, and electrons $T_{1e}$, $T_{2e}^*$, $T_{1\rho e}$. The relaxation curves and corresponding pulse sequences are shown in Fig. S6.

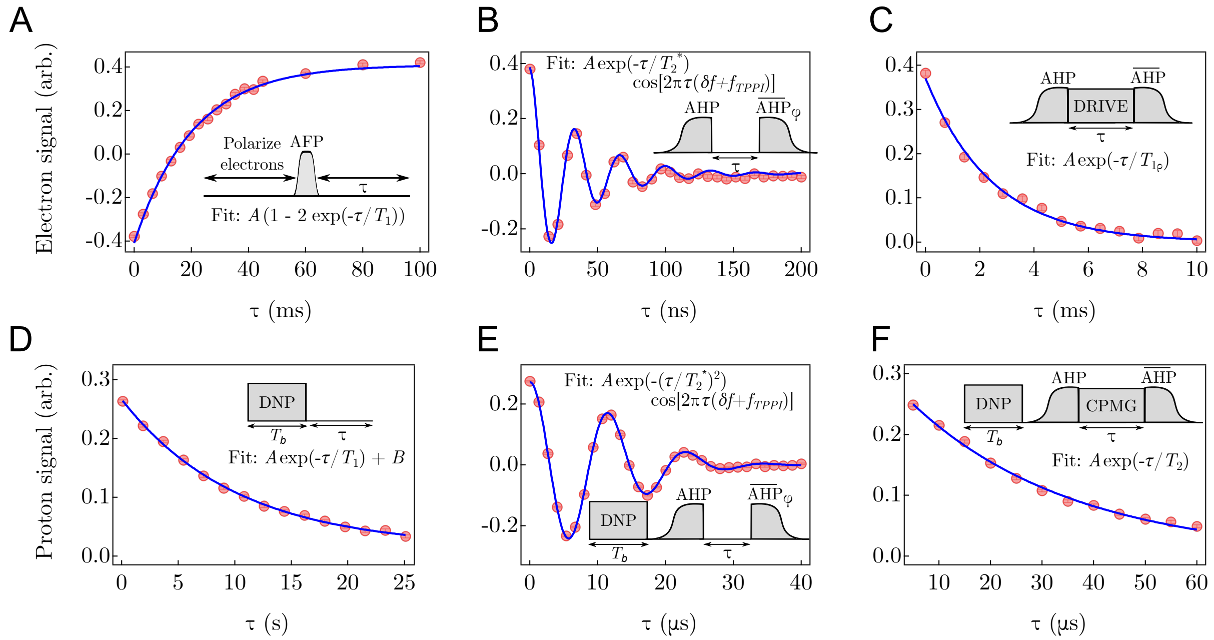


Figure S6: **Relaxation Times.** Spin relaxation data for sample A along with the pulse sequences used to perform the measurements. (**A**) Electron $T_{1e}$ measurement with inversion recovery. (**B**) Electron $T_{2e}^*$ measurement using a modified Ramsey experiment. To enhance sensitivity to the resonance offset, an artificial resonance offset of 30 MHz was introduced using a time-proportional phase increment (TPPI) scheme. (**C**) Electron $T_{1\rho e}$ measurement with a resonant constant-amplitude drive. (**D**) Proton $T_{1p}$ measurement by measuring the decay in the longitudinal magnetization of the hyperpolarized proton ensemble. (**E**) Proton $T_{2p}^*$ measurement using a Ramsey experiment on the hyperpolarized proton ensemble with a TPPI frequency shift of 80 kHz. (**F**) Proton $T_{2p}$ measurement with a $\sigma_z$ decoupling sequence on the proton hyperpolarized ensemble.

$T_{1e}$ was measured using an inversion recovery sequence, wherein the electrons were polarized, and inverted using an AFP. The spins were then allowed to equilibriate for a variable time $\tau$, after which the longitudinal magnetization was measured (Fig. S6A). An exponential fit to the data gives $T_{1e} = 20.5(3)$ ms.

The electron $T_{2e}^*$ was measured using a modified Ramsey experiment with a time-proportional phase-increment (TPPI) scheme. Here, the spins were tipped into the transverse plane using an AHP, followed by a variable free-evolution time $\tau$. Subsequently, an inverse AHP with a phase

Table S2: **Electron and proton relaxation times** for all the measured samples. $T_{2p}$ and $T_{2p}^*$ were not measured for sample D.

| | **Relaxation Time** | **A** | **B** | **C** | **D** |
|---|---|---|---|---|---|
| | $T_{1e}$ (ms) | $20.5(3)$ | $2.5(1)$ | $28.6(7)$ | $30.0(4)$ |
| Electrons | $T_{2e}^*$ (ns) | $38(2)$ | $27(3)$ | $42(2)$ | $50(3)$ |
| | $T_{1\rho e}$ (ms) | $2.5(1)$ | $0.45(4)$ | $3.2(1)$ | $7.5(3)$ |
| | $T_{1p}$ (s) | $10.2(3)$ | $1.01(3)$ | $10.8(6)$ | $20(1)$ |
| Protons | $T_{2p}^*$ ($\mu$s) | $17.0(2)$ | $16.8(2)$ | $16.8(2)$ | - |
| | $T_{2p}$ ($\mu$s) | $31.4(7)$ | $31(1)$ | $30(1)$ | - |

shift $\varphi = 2\pi f_{\mathrm{TPPI}}\tau$ was applied, where $\varphi$ was varied in proportion to $\tau$ to introduce an artificial resonance offset of $f_{\mathrm{TPPI}} = 30$ MHz. The longitudinal magnetization was measured as a function of $\tau$ (Fig. S6B). The artificial offset increases the sensitivity of the measurement to resonance offsets by allowing more oscillations within the signal decay time constant $T_{2e}^*$. A fit with an exponential envelope indicates $\delta f = -144$ kHz and $T_{2e}^* = 38(2)$ ns.

To measure the electron spin-lattice relaxation under constant drive $T_{1\rho e}$, the spins were tipped along the $x$-axis with an adiabatic half-passage (AHP), and then spin-locked with a resonant drive for time $\tau$. An inverse AHP was then applied to bring the spins back to the $z$-axis. The longitudinal magnetization was measured as a function of $\tau$ (Fig. S6C). The $T_{1\rho e}$ obtained from an exponential fit is $2.5(1)$ ms.

The relaxation measurements on proton spins were done after hyperpolarization for increased SNR. Hence, all associated pulse sequences were preceded by the application of DNP to the electron spins for the optimal build-up time $T_{b,\mathrm{opt}}$ given in the main text.

For proton $T_{1p}$, the hyperpolarized proton spins were left to equilibrate for time $\tau$ (Fig. S6D), after which the longitudinal magnetization was measured. An exponential fit to the data gives $T_{1p} = 10.2(3)$ s.

$T_{2p}^*$ was measured similar to $T_{2e}^*$ for hyperpolarized protons with $f_{\mathrm{TPPI}} = 80$ kHz. The data

(Fig. S6) has a Gaussian decay envelope $\propto e^{-(\tau/T_{2p}^*)^2}$, with $\delta f = 5.2$ kHz and $T_{2p}^* = 17.0(2)\ \mu$s from the fit. To measure $T_{2p}$, the spins were tipped to the transverse plane using an AHP, followed by a $\sigma_z$ decoupling sequence consisting of repeated AFPs separated by a free evolution time $\delta\tau = 5\ \mu$s. After the decoupling sequence, an AHP inverse was applied to tip the spins back to the $z$-axis. The total free evolution time $\tau = n\delta\tau$ was varied by incrementing the number $n$ of AFP pulses applied during the decoupling sequence. The longitudinal magnetization was measured as a function of $\tau$ (Fig. S6F). An exponential fit to the data gives $T_{2p} = 31.4(7)\ \mu$s.

# 6 Thermometry

We calibrate the temperature of the SiNW by measuring the power spectral density (PSD) of displacement fluctuations at the mechanical resonance frequency of the SiNW as a function of the incident laser power. The spectral density of thermal force fluctuations on the SiNW is $S_F = 4k_B k T_{\text{NW}}/(\omega_c Q)$, where $k_B$ is the Boltzmann constant, $k$ is the spring constant, $\omega_c$ is the resonance frequency, $Q$ is the native (undamped) quality factor, and $T_{\text{NW}}$ is the temperature of the SiNW. We see that the contribution to the displacement PSD from thermal fluctuations is directly proportional to $T_{\text{NW}}$.

In our experimental setup, the entire system is cooled to a base temperature of $4.2\,\text{K}$. However, the laser shining on the SiNW causes sample heating. To determine the excess heating caused by the laser, the following calibration procedure was performed on the 1.3 mM reference sample: First, the sample was positioned $500\,\text{nm}$ in the $z$ direction away from the constriction and the feedback damping was turned off. Next, the laser was turned on, and a spectrum analyzer was used to measure the total power in 1) A $5\,\text{kHz}$ bandwidth around the NW resonance frequency and 2) A $5\,\text{kHz}$ bandwidth in a background region away from the NW resonance frequency. The background power was then subtracted from the total power in order to obtain the thermal displacement power. The integrated displacement power spectral density is plotted

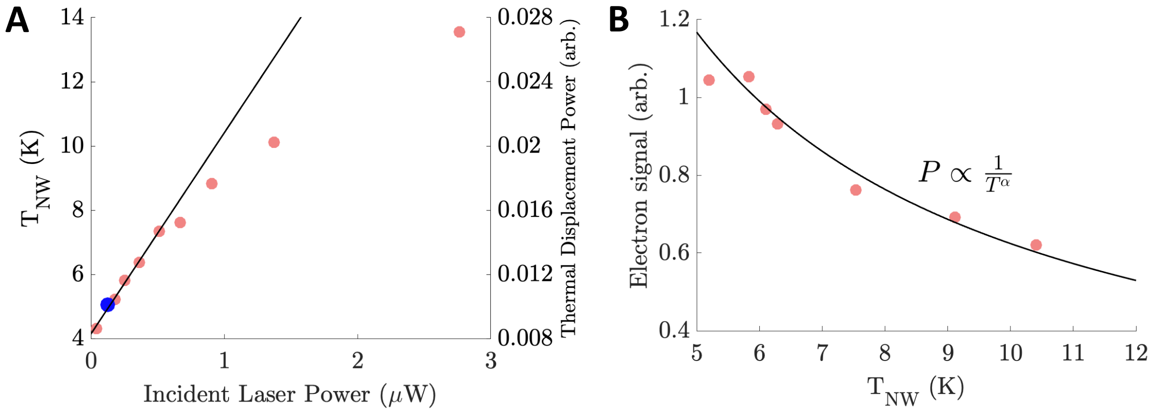


Figure S7: **Thermometry Measurements for the 1.3 mM Reference Sample.** (**A**) (right axis) measured thermal displacement power as a function of the incident laser power, (left axis) extrapolated SiNW temperature. The operating light level of the measurements for this sample is indicated by the blue data point. (**B**) Measurement of the thermal electron spin polarization as a function of the temperature of the SiNW.

as a function of the incident laser power is shown in Fig. S7A. We find that at low light levels, the thermal displacement power increases linearly with the incident laser power. We obtain a calibration of the SiNW temperature by assuming that the $y$ intercept corresponding to the linear part of the curve corresponds to the base temperature of $4.2\,\mathrm{K}$.

As an additional check, we measured the electron spin polarization as a function of the incident laser power. Fig. S7B shows a plot of the electron polarization with the $x$ axis converted to temperature using the data shown in Fig. S7A. We fit the data to a power law $T^{-\alpha}$ and find that the fitted exponent $\alpha = 0.90$ is close to the value $\alpha = 1$, expected from the Curie-Weiss law. Similar measurements on samples A-D revealed a NW temperature of $\sim 6$ K at the operating light level.

# 7 Height dependence of bulk $T_{1e}$

It is known that thermally induced electrical currents (Johnson noise) can cause fluctuating electromagnetic fields close to a conductor, which can increase the spin-lattice relaxation rate (*9*).

To understand whether proximity to the CFFGS contributed to the enhanced electron spin relaxation, we measured $T_{1e}$ as a function of distance from the CFFGS. Fig. S8B shows the $T_{1e}$ values obtained from the fits to the inversion-recovery curves measured for various tip-surface separations. From the data we conclude that there is no discernible change in $T_{1e}$ caused by proximity to the surface of the CFFGS. The lower SNR for the data measured at $528\,\mathrm{nm}$ may be attributed to the decrease in signal resulting from the lower measurement gradients.

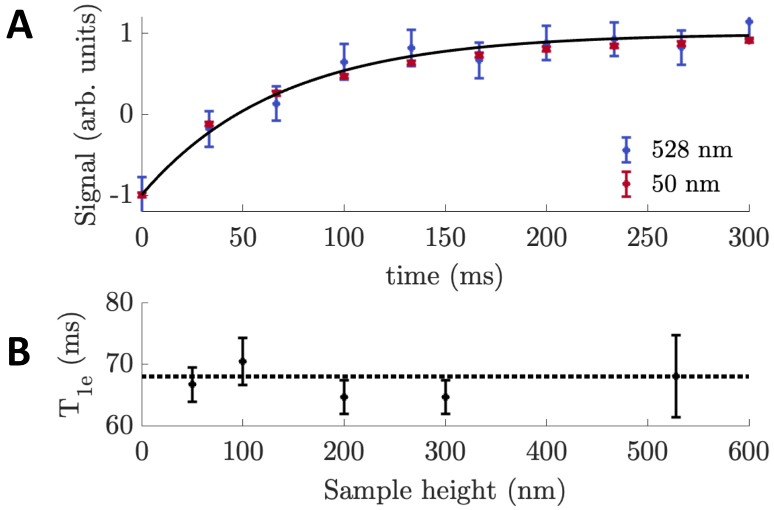


Figure S8: **Effect of Sample Height on Measured Bulk** $T_{1e}$. (**A**) Inversion-recovery curves measured at 50 nm and 528 nm. The black line indicates the fit to a single-exponential decay. Both curves can be fitted by the same $T_{1e} = 70$ ms. (**B**) $T_{1e}$ vs. tip-surface separation.

# 8 Data for Sample B, C, and D

Data for the hyperpolarized and thermal time records, the enhanced signal as a function of the build-up time, and the enhanced signal as a function of $T_{\mathrm{pol}}$ for various $T_{\mathrm{ramp}}$ are shown in Fig. S9, Fig. S10 and Fig. S11.

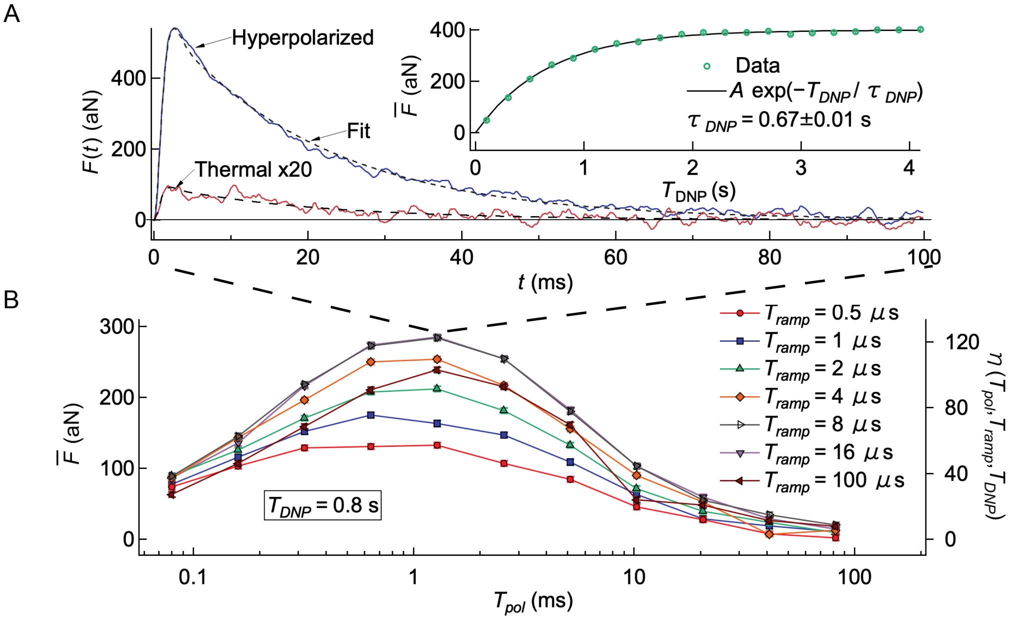


Figure S9: **Sample B Data.** (**A**) Hyperpolarized and thermal time records. The inset shows the enhanced signal as a function of build-up time. **(B)** Measured enhancement and enhanced signal as a function of $T_{\rm pol}$ for various $T_{\rm ramp}$ for a build-up time of 0.8 s.

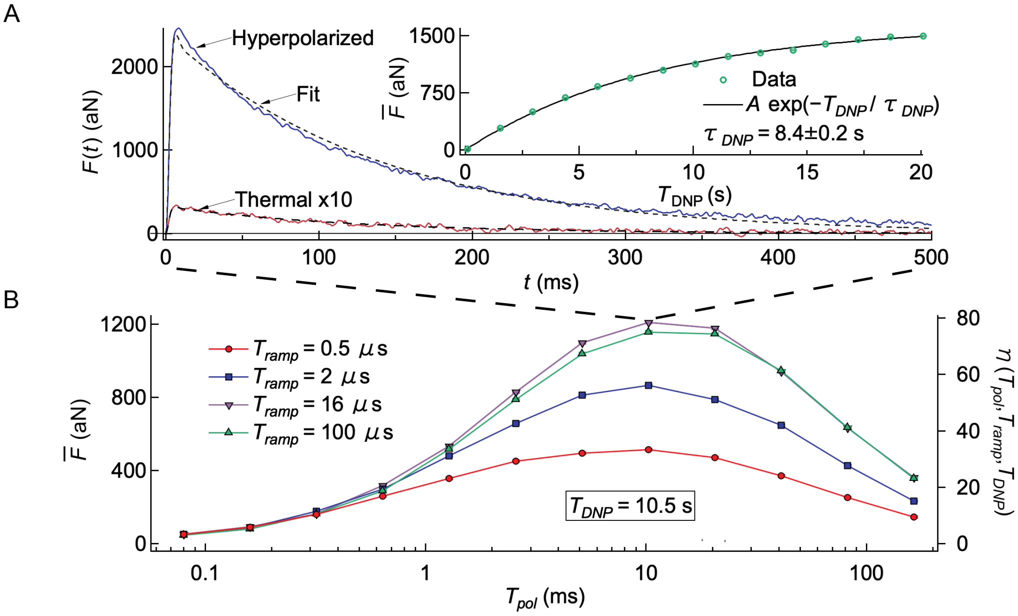


Figure S10: **Sample C Data.** (**A**) Hyperpolarized and thermal time records. The inset shows the enhanced signal as a function of build-up time. **(B)** Measured enhancement and enhanced signal as a function of $T_{\rm pol}$ for various $T_{\rm ramp}$. The build-up time for this sample was 10.5 s.

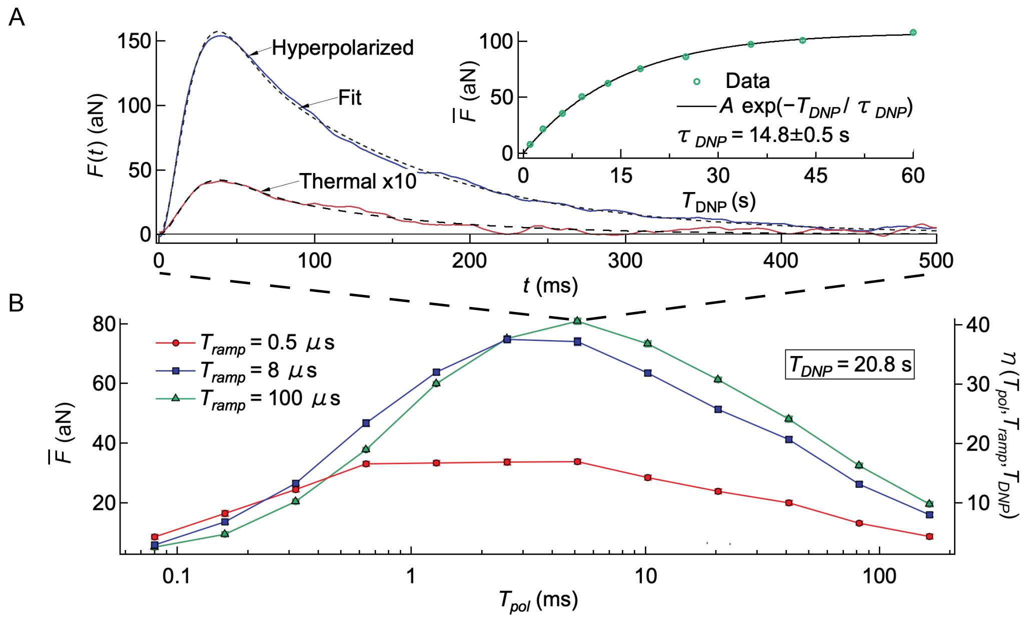


Figure S11: **Sample D Data.** (**A**) Hyperpolarized and thermal time records. The inset shows the enhanced signal as a function of build-up time. **(B)** Measured enhancement and enhanced signal as a function of $T_{\rm pol}$ for various $T_{\rm ramp}$. The build-up time for this sample was 20.8 s.

# 9 DNP Model

Quantitative understanding of the interplay between the various DNP parameters is essential for optimizing the enhancement. We present a semi-classical model for the polarization transfer process in the limit of perfect adiabaticity. During a DNP sweep, for each electron spin, the model randomly chooses a proton spin to interact with from a uniform probability distribution. The electron will then exchange polarization with that proton. We assume that the electron state at the start of each sweep is statistically independent from the previous one. Denoting the number of spin-up (down) protons and electrons before the sweep by $n_{p\uparrow}$ ($n_{e\uparrow}$) and $n_{p\downarrow}$ ($n_{e\downarrow}$), respectively, the average change in the number of spin-up protons is $\delta n_{p\uparrow} = n_{e\uparrow} n_{p\downarrow}/n_p - n_{e\downarrow} n_{p\uparrow}/n_p$, where $n_p$ is the total number of protons. The average change in the proton polarization due to

the transfer $\delta m_{p,\mathrm{tr}} = \delta n_{p\uparrow} - \delta n_{p\downarrow} = 2\delta n_{p\uparrow}$ is thus given by

$$\delta m_{p,\mathrm{tr}} = \frac{2}{n_p}(n_{e\uparrow}n_{p\downarrow} - n_{e\downarrow}n_{p\uparrow}) = m_e - \frac{n_e}{n_p}m_p, \tag{S19}$$

where $m_p$ and $m_e$ are the total proton and electron polarizations before the sweep, respectively, and $n_e$ is the number of electron spins.

There are two contributions to the change in proton polarization $\delta m_p = \delta m_{p,\mathrm{tr}} + \delta m_{p,\mathrm{rel}}$ between two DNP sweeps: 1) transfer of polarization from the electrons $\delta m_{p,\mathrm{tr}}$, and 2) the relaxation of the protons to the lattice $\delta m_{p,\mathrm{rel}}$. Since $T_{\mathrm{pol}} \ll T_{1p}$, the latter is given by $\delta m_{p,\mathrm{rel}} = m_{p0} + (m_p - m_{p0})e^{-T_{\mathrm{pol}}/T_{1p}} \simeq -(T_{\mathrm{pol}}/T_{1p})\,(m_p - m_{p0})$, where $m_{p0}$ is the average proton polarization at thermal equilibrium. By combining this with Eq. S19, we find the rate of change for the proton polarization

$$\dot{m}_p(T_b) \simeq \frac{\delta m_p}{T_{\mathrm{pol}}} = -\left(\frac{n_e}{n_p T_{\mathrm{pol}}} + \frac{1}{T_{1p}}\right) m_p(T_b) + \frac{m_e}{T_{\mathrm{pol}}} + \frac{m_{p0}}{T_{1p}}. \tag{S20}$$

Solving Eq. S20 with the initial condition $m_p(0) = 0$ (due to the scrambling pulse), and conversion to the expected force signal gives

$$\bar{F}_{\mathrm{hp}}(T_b, T_{\mathrm{pol}}, T_{\mathrm{ramp}}) = \bar{F}_{\mathrm{th0}} \frac{1 + r(1 - e^{-T_{\mathrm{pol}}/T_{1e}})\frac{\gamma_e}{\gamma_p}\frac{T_{1p}}{T_{\mathrm{pol}}}}{1 + r\frac{T_{1p}}{T_{\mathrm{pol}}}}\,(1 - e^{-T_b/\tau_{\mathrm{DNP}}}), \tag{S21}$$

with $r = n_e/n_p$, $\tau_{\mathrm{DNP}} = 1/(T_{1p}^{-1} + rT_{\mathrm{pol}}^{-1})$ is the predicted build-up time constant, and $\bar{F}_{\mathrm{th0}} = \bar{F}_{\mathrm{th}}(T_b \to \infty)$ is the force signal at thermal equilibrium. Assuming uniform spin densities, $r$ is equal to the electron-to-proton density ratio.

Using Eq. S21, we conduct a simultaneous fit to the $T_b$- and $T_{\mathrm{pol}}$-dependent data for each sample, with $T_{\mathrm{ramp}} = 100\ \mu$s to ensure sufficient adiabaticity (Fig. S21D,E). The fit parameters are $T_{1e}$ and $r$, which are given in Table S3. For both fits, $T_{1p}$ is held constant at the measured value, which is provided in Table 1 of the main text. The fits are in excellent agreement with the data, and the $T_{1e\,\mathrm{fit}}$ value matches the measured $T_{1e}$ for all samples. To contextualize $r_{\mathrm{fit}}$,

we calculate a range of possible concentration ratios $[r_{\text{min}}, r_{\text{max}}]$ based on the the amount of water remaining in the prepared solution. We observe that for samples B and C, which have the highest OX063 concentrations, $r_{\text{fit}}$ falls below the expected minimum $r_{\text{min}}$. This could be attributed to partial aggregation of OX063 radicals, which can change the spectral properties of the radicals and the number of unpaired electrons. (*10, 11*).

Table S3: **Semi-classical DNP model fit parameters** $T_{1e\text{ fit}}$, $r_{\text{fit}}$ along with the measured $T_{1e}$ and expected proton-to-electron concentration ratios $r$. Maximum and minimum $r$ values are calculated assuming 0% and 100% water retention in the nanodroplets, respectively.

| **Sample** | **A** | **B** | **C** | **D** |
|---|---|---|---|---|
| $T_{1e\text{ fit}}$ (ms) | 22.8(3) | 2.52(5) | 31(1) | 23.4(9) |
| $r_{\text{fit}}$ $(10^{-5})$ | 51.1(6) | 70(2) | 47(2) | 9.1(4) |
| $T_{1e}$ (ms) | 20.5(3) | 2.5(1) | 28.6(7) | 30.0(4) |
| $r_{\text{min}}$ $(10^{-5})$ | 30.6 | 82.9 | 82.9 | 8.98 |
| $r_{\text{max}}$ $(10^{-5})$ | 147 | 351 | 351 | 27.9 |

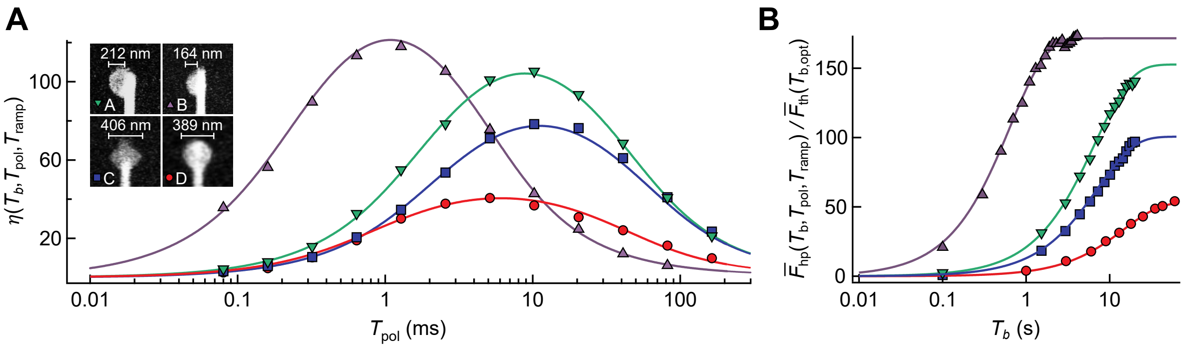


Figure S12: **DNP model fits** for the (**A**) $T_{\text{pol}}$- and (**B**) $T_b$-dependent data. (Inset) SEM images of the nanodroplets attached to each SiNW.

# 10 DNP-Enhanced and Statistical Polarization SNR Comparison for Sample C

Here, we present the comparison of hyperpolarized and statistical SNRs obtained with sample C. The comparison was conducted in the same manner as for sample A presented in the main text. Fourier encoding using the $B_1$ gradient was done using the same $10\ \mu$s resonant pulses discussed in the main text, with the same amplitude sweep. For the hyperpolarized data, the DNP sequence was applied with $T_b = 10.5$ s, with $T_{\text{ramp}} = 16\ \mu$s and $T_{\text{pol}} = 10.24$ ms, after which the proton signal was acquired for 500 ms. Each open circles in Fig. S13C, represents the average of two such measurements, corresponding to a total measurement time of 22.13 s. The statistically-polarized data was obtained by evaluating the force correlation for 100 ms measurement blocks. The solid lines in Fig. S13A,C indicate overall average taken over 15.2 h (statistical) and 2.1 h (hyperpolarized). From the data, we determine $\overline{\text{SNR}}_{\text{st}} = 21.99$ and $\overline{\text{SNR}}_{\text{hp}} = 112.05$ for the statistical and hyperpolarized data, respectively, revealing a reduction in averaging time by a factor of $(\overline{\text{SNR}}_{\text{hp}}/\overline{\text{SNR}}_{\text{st}})^2 \times (15.2\text{ h}/2.1\text{ h}) = 189$ to achieve the same average SNRs.

# 11 Simulation of Surface-Induced Spin Lattice Electron Relaxation

In the main text we mention that fast relaxing paramagnetic defects at the $\text{Si}/\text{SiO}_2$ interface have a role in the $T_{1e}$ relaxation of the bulk trityl-OX063 radicals. Here, we provide the details of the semi-classical spin diffusion simulation used to investigate the role that paramagnetic defects play. The sample geometry is modelled from scanning electron microscope (SEM) images. A random realization of the spin locations is generated inside the geometry based on the expected concentration of trityl radicals and surface defects. Each spin is assumed to be

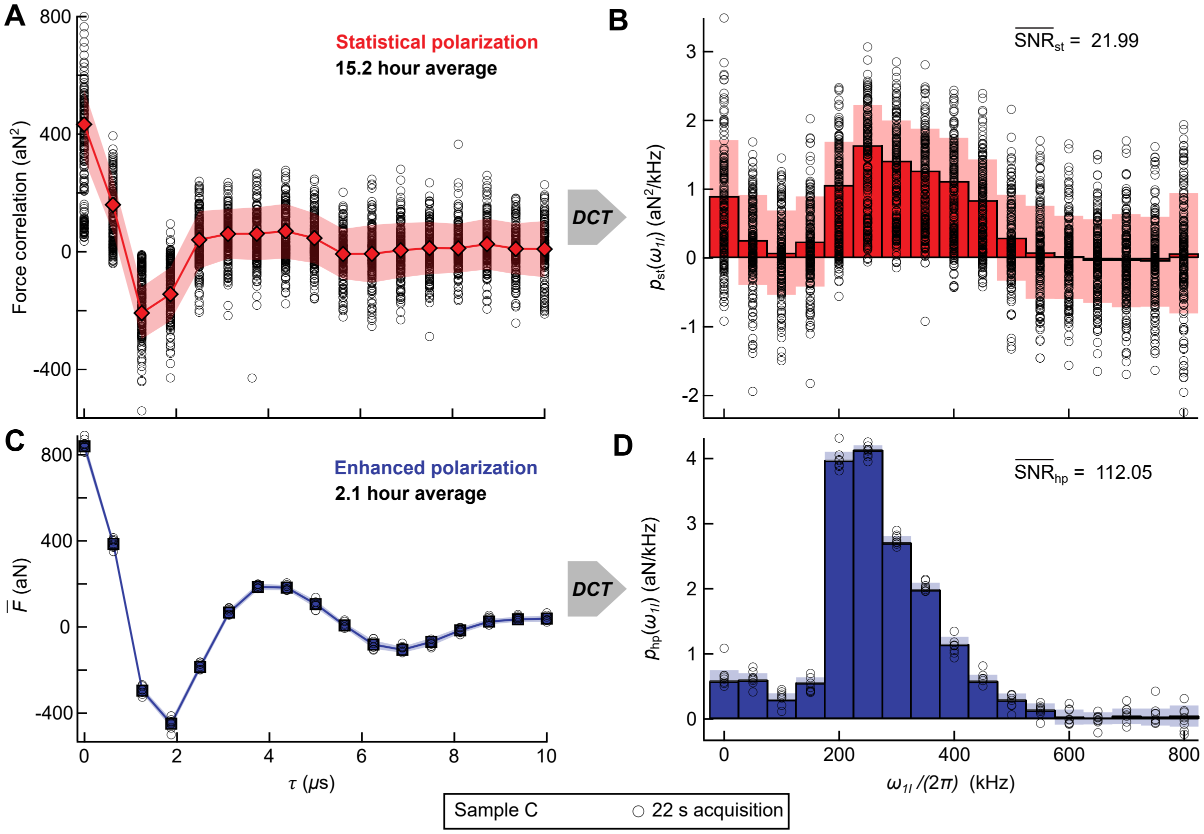


Figure S13: **DNP-Enhanced and Statistical Polarization SNR Comparison for Sample C.** Measured time-domain Fourier encoding data for (**A**) statistically-polarized and (**C**) hyperpolarized proton spins in sample C. The corresponding Rabi frequency distributions are shown in (**B**) and (**D**). Similar to the sample A data (Fig. 5 of the main text), the frequency resolution of each distribution is 50 kHz. The shaded regions indicate the standard deviation of the acquired data (open circles) for each point in the time record.

in either an up or down state. We assume that the evolution of each spin is governed by 1) dipole-dipole interactions with neighbouring spins, and 2) the intrinsic spin-lattice relaxation of the trityl radicals and the fast relaxing paramagnetic defects. We calculate the transition rates due to each of these mechanisms through a perturbative approach and probabilistically evolve the spins accordingly. We simulate the measured $T_{1e}$ relaxation process by calculating the gradient-weighted polarization at each time step.

We begin by first modelling our sample geometry, using the SEM images shown in Fig. 2C

of the main text, to approximate the size and location of the SiNWs and the droplets containing the radicals. We generate a random realization of spin locations by mapping a three-dimensional grid of points onto this geometry, taking a grid spacing $\Delta l = 1\,\mathrm{nm}$. In order to probabilistically populate the grid, we assume that the different points are statistically independent. Each point on the grid is occupied by a spin with a probability of $n_e\ \Delta l^3$ where $n_e$ is the OX063 concentration presented in Table 3 of the main text, assuming zero water content in the droplet. In the $\Delta l \to 0$ limit, the spatial distribution approaches a spatial Poisson process with density $n_e$ (*12*). The fast-relaxing defect spins are assumed to reside in a $1\,\mathrm{nm}$ thick layer on the SiNW; the thickness is chosen to approximate the thickness of the $\mathrm{Si/SiO_2}$ interface. The probability of a point on the grid being occupied by a defect is given as $(\sigma_d/1\,\mathrm{nm})\Delta l^3$, where $\sigma_d$ is the defect density. The simulated relaxation curves, shown in Fig. S14, were calculated for values of $\sigma_d$ in the range of $10^{10}\,\mathrm{cm}^{-2}$ to $10^{14}\,\mathrm{cm}^{-2}$, and different geometries to analyze the role that fast relaxing spins have on spin-lattice relaxation.

A probabilistic approach is taken for modelling the dynamics of the system. Transition rates between spin states are governed by both dipole-dipole interactions between neighboring spins and individual spin-lattice relaxation processes, where the $T_{1e}$ of the bulk spins is assumed to be much longer than those of the fast-relaxing paramagnetic defects. Spin diffusion between electrons is governed by the secular dipolar Hamiltonian which, for a spin pair is $H_D = D(3S_1^zS_2^z - \mathbf{S_1}\cdot\mathbf{S_2})$, where $D = \mu_0\hbar\gamma_e^2(1-3\cos^2\theta)/(4\pi r^3)$ in angular frequency units, $\theta$ is the angle the static field makes with the line connecting the spin pair and $r$ is the distance between the two spins. We can calculate the transition rates from $|{\uparrow\downarrow}\rangle \leftrightarrow |{\downarrow\uparrow}\rangle$ states using Fermi's Golden Rule (*13*). The transition rate $W$ is calculated as

$$W = 2\pi|\langle\uparrow\downarrow|H_D|\downarrow\uparrow\rangle|^2 \int_{-\infty}^{\infty} d\omega\ g_1(\omega)g_2(\omega), \quad \text{(S22)}$$

where $g_1(\omega),\ g_2(\omega)$ are the inhomogeneous normalized lineshapes with $\int_{-\infty}^{\infty} d\omega\ g_i(\omega) = 1$,

$i \in \{1,2\}$. In the simulation, $g(\omega)$ is taken to be a Lorentzian with a full width at half maximum $\delta\omega = 2/T_{2e}^*$. Assuming the distributions are statistically independent, the transition rate evaluates to

$$W = \frac{D^2}{\delta\omega_1 + \delta\omega_2 + 4\frac{(\omega_{01}-\omega_{02})^2}{\delta\omega_1+\delta\omega_2}}, \tag{S23}$$

where $\omega_{01}$ and $\omega_{02}$ are the center frequencies of the bulk and surface spins, respectively, which may be different due to the difference in the distribution of $g$-factors for the two spin species (*14*). The probability for a spin to flip in a time interval $\Delta t$ is $\mathbb{P}(\text{flip}) = W\Delta t$, where $\Delta t$ is the time step in the simulation. We choose $\Delta t$ to be sufficiently small, such that the maximum $\mathbb{P}(\text{flip}) \ll 1$, for all spin pairs in the sample. Because the number of spins in the simulated volume can be quite large ($\sim 700,000$), the computation time becomes impractical when considering the interaction for all spin pairs in the sample. We can reduce the computation time considerably by considering the interaction of only those spins within a "sphere of influence", whose radius is chosen such that the dipole-dipole interaction of the central spin with spins outside the sphere are negligible.

The intrinsic $T_{1e}$ process can also be modelled probabilistically with $\mathbb{P}(|\uparrow\rangle \to |\downarrow\rangle) = (1 - p_e)\Delta t/T_{1e}$, and $\mathbb{P}(|\downarrow\rangle \to |\uparrow\rangle) = p_e\Delta t/T_{1e}$ where $p_e$ is the fractional polarization of spins in the up state at $4\,\text{K}$, and $T_{1e}$ is the intrinsic spin lattice relaxation time of the trityl and defect spins measured in bulk concentrations (*15, 16, 17*).

We assume the initial state of the system to be in a pure state with all spins pointing up. At each time step, we iterate through all spin pairs and calculate the spin-flip probability $\mathbb{P}(\text{flip})$. Then, we generate a random number between 0 and 1. If this number is less than $\mathbb{P}(\text{flip})$ then we flip the states of the spin pair. We then apply the same methodology for a $T_1$ process using probabilities $\mathbb{P}(|\uparrow\rangle \to |\downarrow\rangle)$ and $\mathbb{P}(|\downarrow\rangle \to |\uparrow\rangle)$, with the corresponding $T_{1e}$ for the defect spins and OX063 radicals (*15, 16*). Table S4 provides the details of the parameters used for simulating

samples A, B, and C as well as the $1.3\,\mathrm{mM}$ concentration sample that was used for investigating different electron relaxation mechanisms, referred to as “Reference Sample”. This process is repeated $N$ times with time step $\Delta t = 1\,\mathrm{ns}$. At each time step, we calculate and store the gradient-weighted polarization, which is

$$p(t) = \frac{\begin{bmatrix} S_1(t) & \cdots & S_N(t) \end{bmatrix} \begin{bmatrix} G(\mathbf{r}_1) \\ \vdots \\ G(\mathbf{r}_N) \end{bmatrix}}{\sum_{i=1}^{N} G(\mathbf{r}_i)}, \tag{S24}$$

where $S_i(t) = \pm 1$ refers to the state of the $i^{\text{th}}$ spin in the sample at time $t$. $G(\mathbf{r}_i)$ refers to the detection gradient at the position of the $i^{\text{th}}$ spin, and $N$ is the number of spins in the sample.

Table S4: **Parameters used for Semi-Classical Spin Diffusion Simulations.** Ref. sample refers to the 1.3 mM sample used for investigating different electron relaxation mechanisms.

| **Sample** | **A** | **B** | **C** | **Ref. Sample** |
|---|---|---|---|---|
| Intrinsic $T_{1e\,\mathrm{OX063}}$ (s) | 0.1 | 0.1 | 0.1 | 10 |
| Intrinsic $T_{1e\,\mathrm{defects}}$ (µs) | 50 | 50 | 50 | 50 |
| OX063 Concentration (mM) | 17.8 | 49.4 | 49.4 | 1.3 |
| $T_{2e}^{*}$ OX063 (ns) | 38 | 27 | 42 | 56 |
| $T_{2e}^{*}$ defects (ns) | 12 | 12 | 12 | 12 |

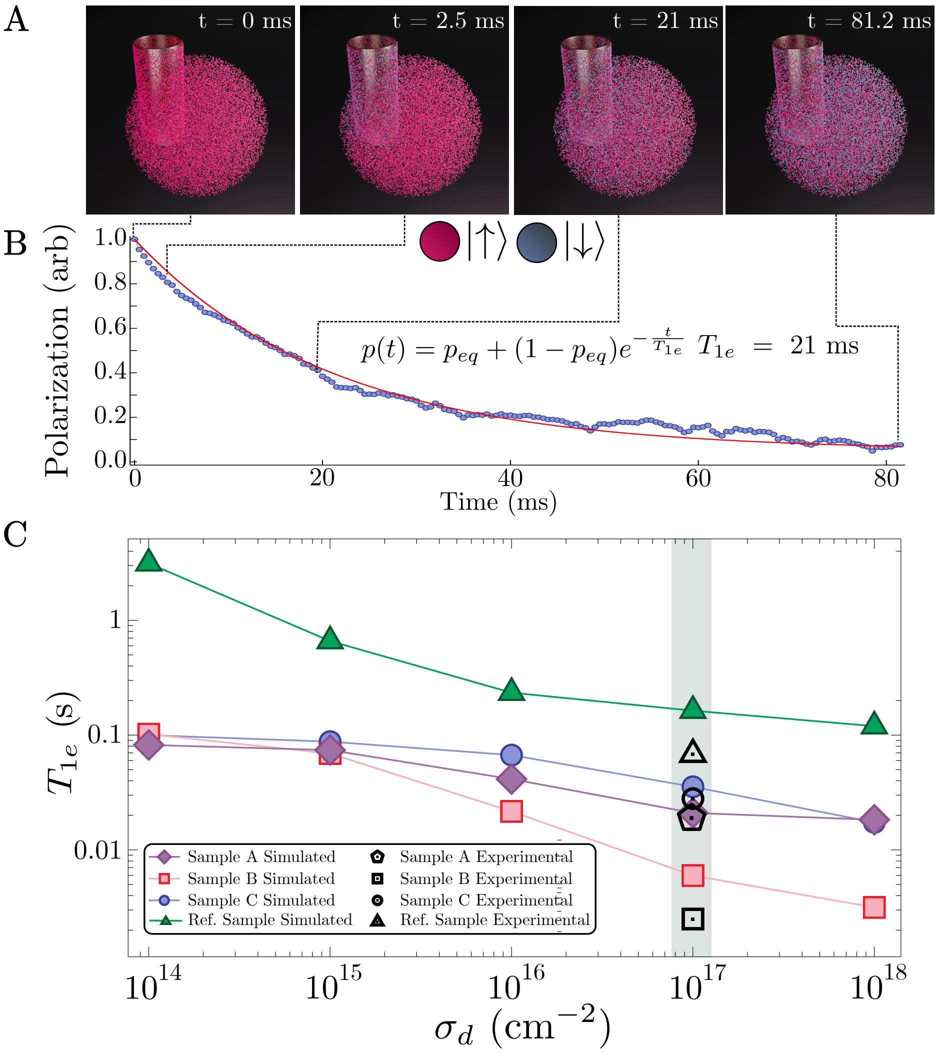


Figure S14: **Spin Diffusion Simulation of Surface Induced Spin Lattice Relaxation**. (**A**) Visualization of spin states at different points in $T_{1e}$ decay for Sample A. At $t = 0$, the sample and surface defects are fully polarized. At $t = 2.5$ ms the fast relaxing spins on the surface of the SiNW have reached thermal equilibrium. At $t = 21$ ms, the bulk polarization has reached the $1/e$ point, and we observe an increase in the number of spins in the down state. At $t = 81.2$ ms ($\sim 3T_{1e}$), the sample has reached thermal equilibrium. (**B**) Sample A fractional polarization time record with spin lattice relaxation time constant $T_{1e} = 21$ ms. (**C**) Spin-lattice relaxation times for samples A, B, and C and the reference sample for different defect densities on the surface of the SiNW.

The results of the simulation are shown in Figure S14, where we have simulated the $T_{1e}$ relaxation for different NW sample geometries for a range of $\sigma_d$. The simulations show good agreement with experimental results for $\sigma_d = 10^{13}\,\mathrm{cm}^{-2}$, which is in the range of the expected defect density reported in literature (*18, 19, 20, 16*). The simulation shows that the presence of fast-relaxing spins of the surface of the SiNW can account for the decrease in $T_{1e}$ of the OX063 radicals observed in our measurements.

# 12 Experimental Setup and Electronics

Fig. S15 shows a schematic of the experimental setup and electronics used for generating spin control and detection pulses for NMR and ESR. A diode laser operating at $\lambda = 1510\,\mathrm{nm}$ is used to detect the displacement of the SiNW. The light exiting the 5% branch of the fiber coupler is focused to a $1.5\,\mu\mathrm{m}$ spot size on the SiNW using a microlens assembly connected to a piezo scanner. The displacement of the SiNW is measured by interfering the back-scattered light from the surface of the SiNW with the light reflected from the cleaved face of the fiber on PD1. The photocurrent generated by PD1 is converted to a voltage using a transimpedance amplifier. The spin signal is obtained by demodulating the voltage signal using a lock-in amplifier referenced to the SiNW frequency (*2*). The light exiting the 95% brach of the fiber coupler is sent to PD2 which is used to monitor the output of the laser diode. The FPGA shown in the figure is responsible for processing the output of the lock-in amplifier as well as sending timing triggers to the arbitrary waveform generators (AWG) and switches. Spin control pulses employed for the MAGGIC protocol and NMR control are driven differentially through the CFFGS using AWG2 and the RF output of AWG1. AWG2 generates the gradient modulation for MAGGIC at the resonant frequency of the SiNW. Meanwhile, the RF output of AWG1 is used to generate pulses at the Larmor frequency of the protons. The output from AWG2 can be switched on or off to gate the power amplifier used for NMR control pulses. Using a passive filter network,

the signal from AWG1 and AWG2 are combined and routed to the low frequency input of the diplexer, which combines the NMR and ESR pulses. The ESR pulses are generated using a single-sideband IQ mixer to up-convert a baseband signal at $374\,\mathrm{MHz}$ from AWG1 to $9.26\,\mathrm{GHz}$. The mixer output is filtered between $9.0\,\mathrm{GHz}$ to $9.4\,\mathrm{GHz}$ to reduce LO leakage and higher order harmonics. To prevent unwanted relaxation caused by the microwave amplifiers, a fast high-power switch is placed before the diplexer to ensure that the amplifier is only on during the application of microwave pulses.

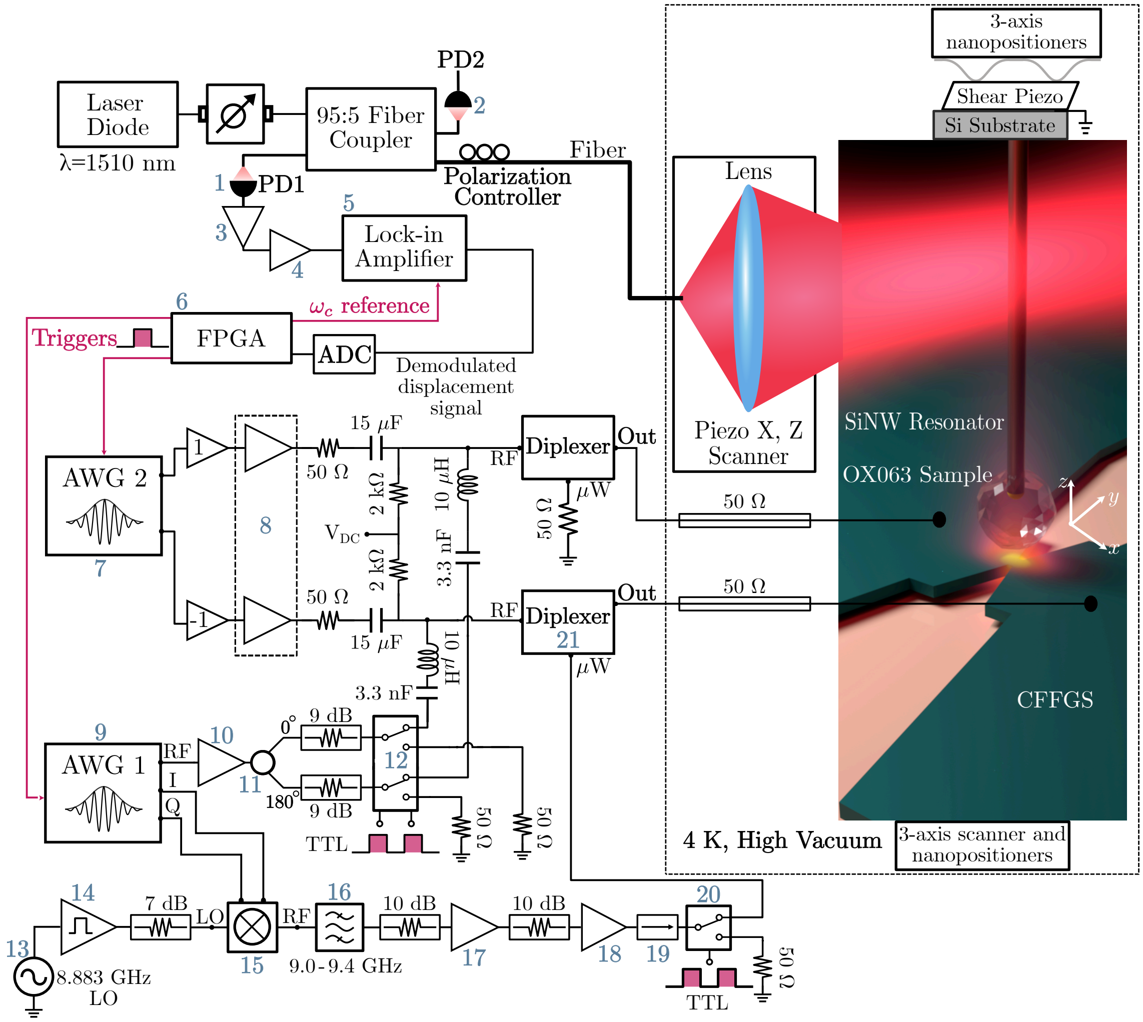


1. PD1: Displacement signal InGaAs photodiode
2. Monitor signal InGaAs photodiode
3. FEMTO DHPCA-100 trans-impedance amplifier
4. SRS Sim910 JFET Preamp
5. SR865 2 MHz DSP lock-in-amplifier
6. NI PXIe-7857R FPGA module
7. NI PXIe-5451 arbitrary waveform generator
8. THS3115 EVM evaluation board
9. Keysight M9336A PXIe I/Q arbitrary waveform generator
10. Mini-Circuits ZHL-32A+ medium high power amplifier
11. TRM Microwave HS155 0/180 hybrid
12. Mini-Circuits ZX80-DR230-S + SPDT RF switch
13. MITEQ DLCRO-010 -08883-3-8P Oscillator
14. Marki AP-0110 broadband distributed amplifier
15. Analog Devices HMC520LC4 GaAs MMIC I/Q Mixer
16. Reactel 8CX1-9200-X400 S11 passband filter
17. B&Z Technologies BZT-08001000-252227-101815 amplifier (Gain: 28dB)
18. Pasternack PE15A4006 1W power amplifier (Gain: 30dB)
19. Fairview Microwave FMIR1027 RF isolator
20. Pasternack PE71S1101 SPDT GaN high power PIN diode switch
21. Mini-Circuits ZDSS-3G-4G-S + diplexer

Figure S15: **Schematic of the Experimental Setup and Electronics.**

# References


1. G. Mathies, S. Jain, M. Reese, R. G. Griffin, *Pulsed Dynamic Nuclear Polarization with Trityl Radicals*. *J. Phys. Chem. Lett.* **7**, 111-116 (2016).

2. H. Haas, S. Tabatabaei, W. Rose, P. Sahafi, M. Piscitelli, A. Jordan, P. Priyadarsi, N. Singh, B. Yager, P. J. Poole, D. Dalacu, R. Budakian, *Nuclear Magnetic Resonance Diffraction with Subangstrom Precision*. *Proc. Natl. Acad. Sci. U.S.A* **119**, e2209213119 (2022).

3. W. Rose, H. Haas, A. Q. Chen, N. Jeon, L. J. Lauhon, D. G. Cory, R. Budakian, *High-Resolution Nanoscale Solid-State Nuclear Magnetic Resonance Spectroscopy*. *Phys. Rev. X* **8**, 011030 (2018).

4. S. Tabatabaei, H. Haas, W. Rose, B. Yager, M. Piscitelli, P. Sahafi, A. Jordan, P. J. Poole, D. Dalacu, R. Budakian, *Numerical Engineering of Robust Adiabatic Operations*. *Phys. Rev. Appl.* **15**, 044043 (2021).

5. G. Turin, *An Introduction to Matched Filters*. *IRE Trans. Inf. Theory IEEE* **6**, 311-329 (1960).

6. J. M. Nichol, T. R. Naibert, E. R. Hemesath, L. J. Lauhon, R. Budakian, *Nanoscale Fourier-Transform Magnetic Resonance Imaging*. *Phys. Rev. X* **3**, 031016 (2013).

7. M. B. Priestley, *Spectral Analysis and Time Series*, vol. 1 (1981).

8. M. S. Bartlett, *On the Theoretical Specification and Sampling Properties of Autocorrelated Time-Series*. *J. R. Stat. Soc.* **8**, 27–41 (1946).

9. S. Kolkowitz, A. Safira, A. A. High, R. C. Devlin, S. Choi, Q. P. Unterreithmeier, D. Patterson, A. S. Zibrov, V. E. Manucharyan, H. Park, M. D. Lukin, *Probing Johnson Noise and*

*Ballistic Transport in Normal Metals with a Single-Spin Qubit*. *Science* **347**, 1129-1132 (2015).

10. I. Marin-Montesinos, J. C. Paniagua, M. Vilaseca, A. Urtizberea, F. Luis, M. Feliz, F. Lin, S. Van Doorslaer, M. Pons, Self-assembled trityl radical capsules – implications for dynamic nuclear polarization. *Phys. Chem. Chem. Phys.* **17**, 5785-5794 (2015).
11. R. Shankar Palani, M. Mardini, Y. Quan, R. G. Griffin, Dynamic nuclear polarization with trityl radicals. *Journal of Magnetic Resonance* **349**, 107411 (2023).
12. A. Papoulis, S. Pillai, *Probability, Random Variables, and Stochastic Processes* (McGraw-Hill, 2002).
13. N. Bloembergen, *On the Interaction of Nuclear Spins in a Crystalline Lattice*. *Physica* **15**, 386-426 (1949).
14. A. Baumer, M. Stutzmann, M. S. Brandt, F. C. Au, S. T. Lee, *Paramagnetic Defects of Silicon Nanowires*. *Appl. Phys. Lett.* **85**, 943-945 (2004).
15. H. Chen, A. G. Maryasov, O. Y. Rogozhnikova, D. V. Trukhin, V. M. Tormyshev, M. K. Bowman, *Electron Spin Dynamics and Spin–Lattice Relaxation of Trityl Radicals in Frozen Solutions*. *Phys. Chem. Chem. Phys.* **18**, 24954-24965 (2016).
16. A. Stesmans, *The .Si Identical to $Si_3$ Defect at Various (111)Si/SiO2 and (111) $Si/Si_3N_4$ Interfaces*. *Semicond. Sci. Technol.* **4**, 1000 (1989).
17. J. Dalibard, Y. Castin, K. Mølmer, *Wave-Function Approach to Dissipative Processes in Quantum Optics*. *Phys. Rev. Lett.* **68**, 580–583 (1992).
18. K. L. Brower, T. J. Headley, *Dipolar Interactions Between Dangling Bonds at the (111) $Si$-$SiO_2$ Interface*. *Phys. Rev. B* **34**, 3610–3619 (1986).

19. B. Nouwen, A. Stesmans, *Dependence of Strain at the (111) Si/SiO$_2$ Interface on Interfacial Si Dangling-Bond Concentration*. *Mater. Sci. Eng., A* **288**, 239-243 (2000).

20. R. Rurali, *Colloquium: Structural, Electronic, and Transport Properties of Silicon Nanowires*. *Rev. Mod. Phys.* **82**, 427–449 (2010).
